# Supplementary material for: Small Scale Data-Free Knowledge Distillation
Source: arXiv:2406.07876 source file (2024-06-12)
Supplement: Supplementary file 1 [file X_suppl.tex]

\clearpage
\newpage
\onecolumn
\appendix
\setcounter{page}{1}
\setcounter{section}{0}
\maketitlesupplementary

\section{Experimental setup}

%We provide the hyper-parameters of training small scale data-free knowledge distillation in Table 
We provide training settings of the teacher w.r.t different datasets in Table \ref{tab:training-setting}. The cos in the table means setting the learning rate of each parameter group using a cosine annealing schedule.

We only use the test dataset for testing and it is not accessible to the training dataset. However, the data samples are the same as the synthetic replay buffer for knowledge distillation. We use random crop with padding 4 and random horizontal flip for data augmentation in both classification and segmentation datasets. 

\section{Effects of $\gamma$}
We conduct the robustness testing on the hyper-parameter about $\gamma$ as shown in Figure \ref{fig:gamma}. We change the hyper-parameter $\gamma$ from 1 to 9. Our method shows the best performance around values 4.

\begin{figure}[t]
    \centering
    \begin{tabular}{c}
    \includegraphics[width=0.65\linewidth]{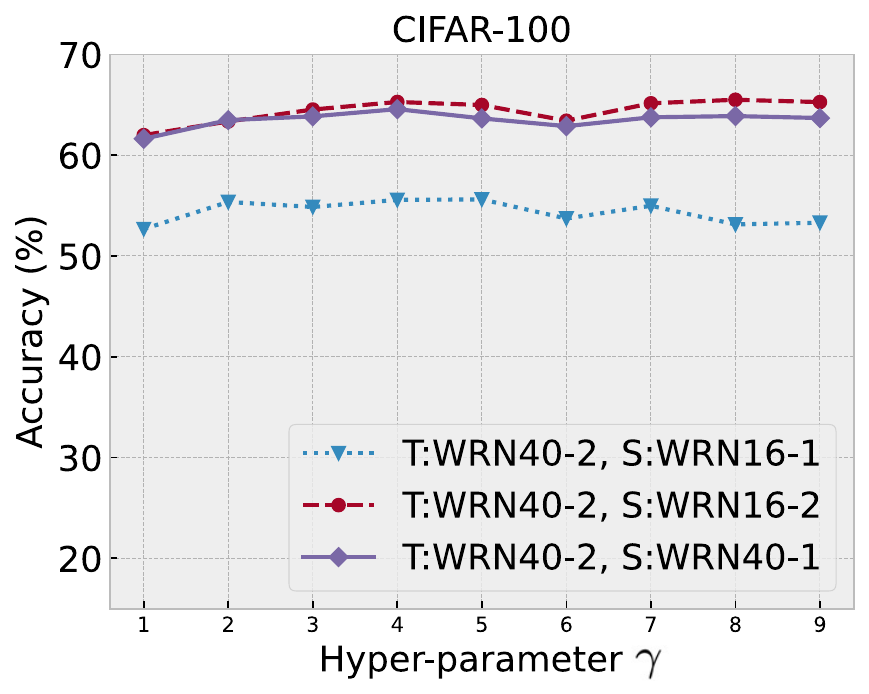} \\
    \end{tabular}
    \centering
    % \vspace{0.15in}
    \caption{Classification accuracy of SSD-KD with $\gamma$.}
    \label{fig:gamma}
    \vspace{-1.em}
\end{figure}

\section{More visualization}

We also visualize some synthetic data conducted on the CIFAR-10 and CIFAR-100 dataset inverted by D-KD and our SSD-KD as shown in Figure \ref{fig:vis111} and Figure \ref{fig:vis222}.

\begin{figure}[t]
    \centering
    \begin{tabular}{c c}
    \includegraphics[width=0.45\linewidth]{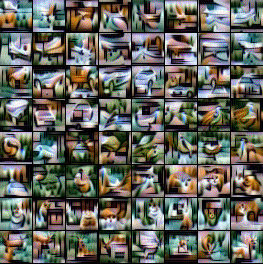}&%
        \includegraphics[width=0.45\linewidth]{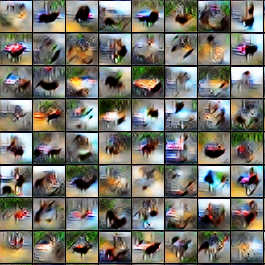} \\%
    \end{tabular}
    \centering
    \vspace{0.10in}
    % \caption{The synthetic data conducted on the CIFAR-10 dataset is inverted by D-KD and our SSD-KD, and is represented across two figures. Images in the left and right figures are inverted by the D-KD and our SSD-KD, respectively. The visualization results show that our method can invert more texture and semantic information with small-scale synthetic data.}
    \caption{Visualization examples of synthetic image samples generated by DeepInv (Left) and our SSD-KD (Right) for the CIFAR-10 dataset.}
    \label{fig:vis111}
    \vspace{-1.em}
\end{figure}

\begin{figure}[t]
    \centering
    \begin{tabular}{c c}
    \includegraphics[width=0.45\linewidth]{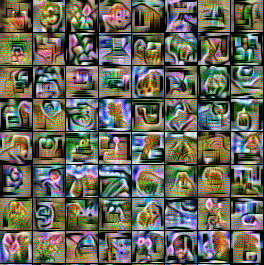}&%
        \includegraphics[width=0.45\linewidth]{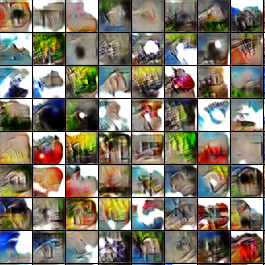} \\%
    \end{tabular}
    \centering
    \vspace{0.10in}
    % \caption{The synthetic data conducted on the CIFAR-100 dataset inverted by D-KD and our SSD-KD, as represented across two figures. The left and right figure is inverted by the D-KD and our SSD-KD, respectively. The visualization results show that our method can invert more texture information and more semantic information with small-scale synthetic data.}
    \caption{Visualization examples of synthetic image samples generated by DeepInv (Left) and our SSD-KD (Right) for the CIFAR-100 dataset.}
    \label{fig:vis222}
    \vspace{-1.em}
\end{figure}

% Please add the following required packages to your document preamble:
% \usepackage{multirow}
\begin{table*}[t]
\setlength{\abovecaptionskip}{0.1in}
\centering
\vspace{-1.em}
\caption{Training settings of teacher w.r.t different datasets. Different meanings of abbreviations: opt: optimizer, wd: weight decay, mo: momentum, bs: batch size, ls: scaling learning rate or not with the base batch size of 256, ld: the method of scaling learning method, ldep: maximum number of iterations of scaling learning method, eta\_min: minimum learning rate of scaling learning method, ep: total number of epochs, wep: number of warm-up epochs.}
\resizebox{0.65\linewidth}{!}{%
\begin{tabular}{cccccccccccc}
\toprule[1.2pt]
\multirow{2}{*}{Dataset} & \multicolumn{11}{c}{Training settings}                                 \\ \cline{2-12} 
                         & opt & lr  & wd   & mo  & bs  & ls  & ld  & ldep & eta\_min & ep  & wep \\ \hline
CIFAR-10                 & SGD & 0.1 & 1e-4 & 0.9 & 256 & yes & cos & 200  & 2e-4     & 200 & 0   \\
CIFAR-100                & SGD & 0.1 & 1e-4 & 0.9 & 256 & yes & cos & 200  & 2e-4     & 200 & 0   \\
NYUv2                    & SGD & 0.1 & 5e-5 & 0.9 & 64  & yes & cos & 190  & 1e-4     & 250 & 0   \\ 
\toprule[1.2pt]
\end{tabular}
\label{tab:training-setting}
}
\vspace{-1.em}
\end{table*}
